# Supplementary material for: SCOPE: Secure Compiling of PLCs in Cyber-Physical Systems
Source: arXiv:2012.12529 source file (2021-11-22)
Supplement: Supplementary file 1 [file 13_appendix.tex]

\section{Appendix}
\appendix
